# Supplementary material for: HarmonySeg: Tubular Structure Segmentation with Deep-Shallow Feature Fusion and Growth-Suppression Balanced Loss
Source: arXiv:2504.07827 source file (2025-04-10)
Supplement: Supplementary file 1 [file X_suppl.tex]

% \iffalse 
\clearpage
\setcounter{page}{1}
\maketitlesupplementary
